# Supplementary material for: Absence of Local Fluctuating Dimers in Superconducting Ir$_{1-x}$(Pt,Rh)$_x$Te$_2$
Source: arXiv:1801.00050 source file (2017-12-29)
Supplement: Supplementary file 1 [file IrTe2-noQCP-supplement.pdf]

# Supplemental Material
# Absence of Local Fluctuating Dimers in Superconducting $Ir_{1-x}(Pt,Rh)_xTe_2$


Runze Yu,[1,†] S. Banerjee,[2] H. Lei,[1,††] Ryan Sinclair,[3] M. Abeykoon,[4]
H. D. Zhou,[3] C. Petrovic,[1] Z. Guguchia,[1,5] and E. S. Bozin[1,*]

[1] *Condensed Matter Physics and Materials Science Department, Brookhaven National Laboratory, Upton, NY 11973, USA**
[2] *Department of Applied Physics and Applied Mathematics, Columbia University, New York, NY 10027, USA*
[3] *Department of Physics and Astronomy, University of Tennessee, Knoxville, Tennessee 37996, USA*
[4] *Photon Sciences Division, Brookhaven National Laboratory, Upton, NY 11973, USA and*
[5] *Department of Physics, Columbia University, New York, NY 10027, USA*


## SAMPLE CHARACTERIZATION

Temperature dependent electrical transport and magnetization measurements on the samples used in this study were carried out on warming in *Quantum Design* PPMS-9 and MPMS-XL5. Results are shown in Fig. S 1. There is a clear anomaly seen in the parent $IrTe_2$ associated with a simultaneous structural and electronic phase transition where long range dimer order is established. No such anomalies are seen in the data for Pt and Rh substituted samples $Ir_{0.95}Pt_{0.05}Te_2$ and $Ir_{0.8}Rh_{0.2}Te_2$, implying the absence of a dimerization transition for these compositions. On the other hand, the low temperature resistivity and susceptibility data shown in the insets to the figure clearly demonstrate bulk superconductivity of our samples (vertical arrows indicate $T_c$).

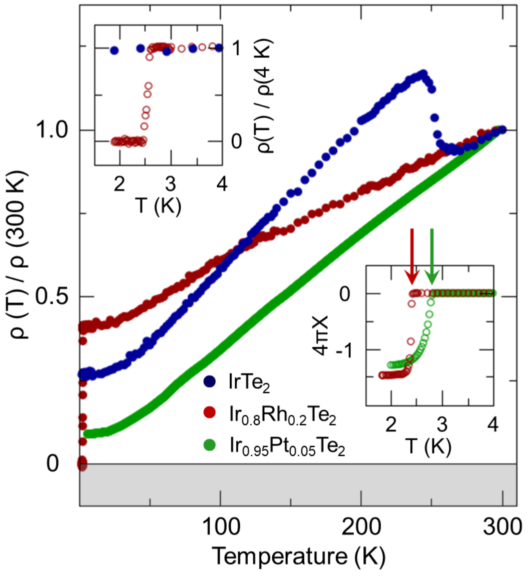


**Figure S** 1. (Color online) Electrical resistivity of $IrTe_2$, $Ir_{0.95}Pt_{0.05}Te_2$, and $Ir_{0.8}Rh_{0.2}Te_2$ samples, normalized to their 300 K value. Insets: (upper left corner) low temperature resistivity, and (lower right corner) low temperature susceptibility collected in the zero field cooling mode.

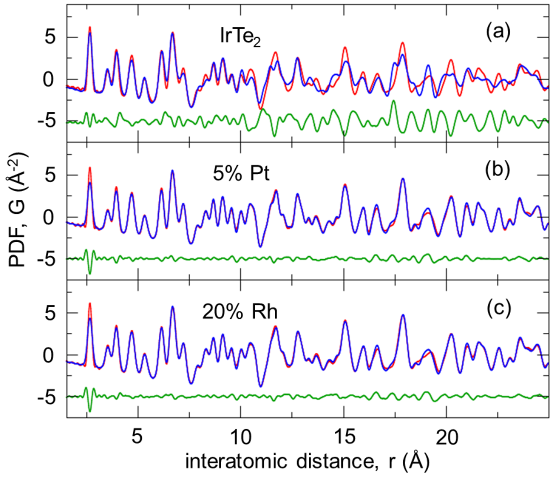


**Figure S** 2. (Color online) A comparison of the 10 K (blue) and 300 K (red) PDF data for (a) $IrTe_2$, (b) $Ir_{0.95}Pt_{0.05}Te_2$, and (c) $Ir_{0.8}Rh_{0.2}Te_2$, where the 10 K data were adjusted in a simple optimization procedure described in the text. Differences are plotted underneath and offset for clarity.

## MODEL INDEPENDENT VERIFICATION OF LOCAL SYMMETRY BREAKING

Figure S 2 summarizes the comparisons of qualitative features of the 10 K and 300 K PDF data for the three samples used in our study. For the comparisons, the low temperature PDF profiles were subjected to a simple semiempirical protocol, dubbed morphing and described briefly below. The morphing analysis indicates that, while symmetry breaking is required to explain the differences observed in the $IrTe_2$ data, the differences observed in the $Ir_{0.95}Pt_{0.05}Te_2$ and $Ir_{0.8}Rh_{0.2}Te_2$ data are likely due to mundane thermal effects only.

The morphing comparison procedure allows for an assessment of similarities of two sets of PDF data to be carried out without an assumption of any specific structure model. This allows, at least in principle, a differentiation between symmetry breaking effects and trivial lattice expansion effects as sources of the observed differences, such as those shown in Fig. 2(d)-(f) of the main text. In

the PDF morphing protocol one of the two experimental PDF profiles to be compared is selected as a target (or a reference), and is not being altered in any way. The target PDFs selected here are the 300 K data. The other of the two profiles to be compared is then taken as a morphing subject, that is to be morphed into the target PDF. In our case these are the 10 K data. The morphing is parametrized by three variables - horizontal and vertical linear scale factors, which stretch the $r$ and $G$ axes respectively, and a "smear" parameter that convolutes the morphing subject with a Gaussian of fixed width. A least squares optimization protocol utilizing these three variables is then carried out until the best possible match between the morph PDF and the target PDF is achieved. This is quantified by minimizing the weighted residual, $r_w$, of the PDF difference and by maximizing the Pearson correlation coefficient, $P$. In the case of ideal morphing $r_w$ would be 0, whereas $P$ would take a value of 1, reflecting perfect agreement between the morph and the target PDF and a 100% positive correlation between the two profiles whose similarity is being evaluated. Elaborating on mathematical treatment and more involved details of this protocol is beyond the scope of this study and will be reported elsewhere (S. J. L. Billinge et al., unpublished).

When the difference between the two measured PDFs originates just from trivial lattice effects, such as thermal expansion, then the morphing procedure can be successful, as would be reflected in a low value of $r_w$ and the Pearson correlation coefficient close to 1. Conversely, when the difference between the two experimental PDFs originates from more complex effects, such as the effects of symmetry breaking, the morphing procedure would fail, resulting in suboptimal $r_w$ and $P$. To benchmark the comparison of the 10 K and 300 K PDF data (Fig. 2(d)-(f) of the main text) when no morphing is applied, we calculated ($r_w$, $P$) pairs for all three samples studied. This benchmarking yields (0.52, 0.86), (0.65, 0.89), and (0.56, 0.91) for $IrTe_2$, $Ir_{0.95}Pt_{0.05}Te_2$, and $Ir_{0.8}Rh_{0.2}Te_2$, respectively. The fully converged morphing process yields (0.46, 0.89), (0.14, 0.99), and (0.15, 0.99), for $IrTe_2$, $Ir_{0.95}Pt_{0.05}Te_2$, and $Ir_{0.8}Rh_{0.2}Te_2$, respectively. Formal comparison of the observed $r_w$ and $P$ values to the benchmark references reveals that these parameters improve considerably by morphing in the case of $Ir_{0.95}Pt_{0.05}Te_2$ and $Ir_{0.8}Rh_{0.2}Te_2$, but do not improve much at all for the $IrTe_2$ parent. This is also reflected in the corresponding difference curves shown in Figure S 2. Our analysis suggests that the difference in PDFs for SC samples is likely caused only by simple lattice effects without any symmetry breaking. Further confidence in the conclusions derived from this analysis comes from the fact that it successfully singles out a symmetry breaking in $IrTe_2$, as is expected when comparing the two datasets straddling the structural transition. In such a case, morphing fails and results in a high value of the weighted residual and the correlation factor much lower than one, without observable improvement by the morphing.

Although the morphing of the data for the SC samples is reasonably good, it is observably non-ideal, as evident from a careful inspection of the difference curves shown in Fig. 2 (b) and (c). While the discrepancies could indicate underlying symmetry breaking, the more likely reason behind this lies in the oversimplifications upon which the morphing algorithm is based. The three parameters allowing for scaling, stretching, and smearing of the subject PDF profile effectively mimic only spherically uniform and isotropic thermal effects, whereas in a real material thermal expansion and thermal vibrations have more complex impact on the PDF profile. Further, the largest discrepancies in the differences observed in Fig. 2 (b) and (c) are confined to a narrow $r$-range just underneath the first PDF peak around 2.5 Å, the region known to be affected by the effects of the correlated motion of the nearest neighbors [1]. The morphing protocol used here does not account for this effect in any way. Considering these shortcomings, and despite them, the morphing analysis rather intuitively suggests that the local symmetry breaking associated with dimer fluctuations at low temperature is highly unlikely.

* bozin@bnl.gov
† Present address: Institute of Physics, Chinese Academy of Science, Beijing, 100190, Peoples Republic of China
†† Present address: Department of Physics, Renmin University, Beijing 100872, Peoples Republic of China

[1] T. Egami and S. J. L. Billinge, *Underneath the Bragg peaks: structural analysis of complex materials* (Elsevier, Amsterdam, 2012), 2nd ed., URL `http://store.elsevier.com/product.jsp?lid=0\&iid=73\&sid=0\&isbn=9780080971414`.
